# Supplementary material for: Data Mining in Transportation Networks with Graph Neural Networks: A Review and Outlook
Source: arXiv:2501.16656 source file (2025-01-28)
Supplement: Supplementary file 1 [file appendix.tex]

\appendix
\newpage 
\begin{appendices}
\section{Survey table}
\begin{table}[H]
\centering
\resizebox{0.95\textwidth}{59mm}{
\begin{tabular}{@{}llr@{}}
\toprule[1.2pt]
\addlinespace[6pt]
Survey question                                                           & Variable      & Value          \\ \addlinespace[4pt] \hline
\addlinespace[6pt]
What is your age?       & $q_{age}$    & >0  \\
\addlinespace[4pt]
What is your sex?   & $q_{sex}$    & 0, 1 (0: female; 1: male) \\
\addlinespace[4pt]
Did you own or rent your house?  & $q_{house}$  & 0, 1 (0: rent; 1: own)   \\
\addlinespace[4pt]
Which ethnic groups do you belong to?                                       & $q_{race}$   & \begin{tabular}[c]{@{}l@{}}Seven groups: African American; \\ Asian/Pacific Islander; Caucasian; Hispanic; \\ Native American; Multiple/mixed; Others\end{tabular} \\
\addlinespace[4pt]
What is your yearly household income?                                                         & $q_{income}$    & \begin{tabular}[c]{@{}l@{}}Nine intervals: <\$15K; \$15-30K; \$30-45K;\\ \$45-60K; \$60-75K; \$75-90K; \$90-105K;\\ \$105-120K; >\$120K    \end{tabular} \\
\addlinespace[4pt]
\begin{tabular}[c]{@{}l@{}}To what extent have the following people returned?\\ \;\;\;a. your neighborhoods \\ \;\;\;b. others in your community\end{tabular} & \begin{tabular}[c]{@{}l@{}}\\$q_{human,\;a}$\\$q_{human,\;b}$\\\end{tabular}  & 0$-$1 (0: not return; 1: full return)\\ 
\addlinespace[4pt]
\begin{tabular}[c]{@{}l@{}}To what extent have the following organizations reopened?\\\;\;\;a. medical facilities\\ \;\;\;b. school/childcare\\ \;\;\;c. businesses\\ \;\;\;d. your employer\\ \;\;\;e. other community\end{tabular}                 & \begin{tabular}[c]{@{}l@{}}\\
$q_{social,\;a}$\\
$q_{social,\;b}$\\
$q_{social,\;c}$\\
$q_{social,\;d}$\\
$q_{social,\;e}$\end{tabular}  & 0$-$1 (0: not reopen; 1: full reopen) \\  \addlinespace[4pt]
\begin{tabular}[c]{@{}l@{}}To what extent has your community experienced recovery?\\
\;\;\;a. power\\
\;\;\;b. water/sewer\\
\;\;\;c. roads/highways\\
\;\;\;d. bridges\\
\;\;\;e. buildings/structures\end{tabular}                 & \begin{tabular}[c]{@{}l@{}}\\
$q_{physical,\;a}$\\
$q_{physical,\;b}$\\
$q_{physical,\;c}$\\
$q_{physical,\;d}$\\ $q_{physical,\;e}$\end{tabular} & 0$-$1 (0: complete damage; 1: full function)   \\ \addlinespace[4pt]
Did you evacuate?                   & $y_{evacuate}$    & 0, 1 (0: not evacuate; 1: evacuate) \\ \addlinespace[4pt]
Have you returned home permanently? & $y_{return}$    & 0, 1 (0: not return; 1: return)    \\ \addlinespace[4pt]
\bottomrule[1.2pt]                       
\end{tabular}}
\caption{\label{table_variable} \footnotesize Variables mined from the THRS.}
\end{table}
\section{Code structure}
\begin{figure}[H]
    \centering
    \includegraphics[scale=0.52]{figure/code_structure_20231222.jpg}
    \caption{The flowchart of DIRSIM.}
    \label{fig16}
\end{figure}

\end{appendices}
